# Supplementary material for: A multi-modal infant-based metric for choosing the best supernova
Source: arXiv:2504.00902 source file (2025-04-01)
Supplement: Supplementary file 1 [file appendix.tex]

\section{Helpful thing 1}
